# Supplementary material for: Modeling Between-Study Heterogeneity for Improved Reproducibility in Gene Signature Selection and Clinical Prediction
Source: arXiv:1708.05508 ancillary file (2019-03-26)
Supplement: Supplementary file 1 [file supplementaryv2.pdf]

# Supplemental Material for “Modeling Between-Study Heterogeneity for Improved Replicability in Gene Signature Selection and Clinical Prediction”

Naim U. Rashid<sup>1,2</sup>, Quefeng Li<sup>1</sup>, Jen Jen Yeh<sup>2,3,4</sup>, and Joseph G. Ibrahim<sup>1</sup>

February 17, 2019

<sup>1</sup>Department of Biostatistics, Gillings School of Global Public Health

<sup>2</sup>Lineberger Comprehensive Cancer Center

<sup>3</sup> Department of Surgery

<sup>4</sup> Department of Pharmacology

University of North Carolina at Chapel Hill

Chapel Hill, NC, U.S.A.

Naim U. Rashid [naim@unc.edu](mailto:naim@unc.edu),

Quefeng Li [quefeng@email.unc.edu](mailto:quefeng@email.unc.edu),

Jen Jen Yeh [jen\\_jen\\_yeh@med.unc.edu](mailto:jen_jen_yeh@med.unc.edu), and

Joseph G. Ibrahim [ibrahim@bios.unc.edu](mailto:ibrahim@bios.unc.edu)

# S1 TSP construction and screening

We provide a new comprehensive workflow of TSP construction and screening. Because the number of gene pairs grows fast with the number of genes, it is preferable to filter genes prior to gene pair construction. Inspired by Afsari et al. (2015), we focus on genes differentially expressed (DE) between subtypes. We first utilize the Wilcoxon Rank Sum Test to determine whether a gene is differentially expressed in one study. To avoid the uncertainty of whether between-sample normalization procedure is performed, we rank transform columns of the expression data matrix before carrying out the Wilcoxon Rank Sum Test gene by gene. Then we sum up the negative logarithm of the p-values from the four studies and keep 75% genes with the smallest overall p-values.

After applying this approach, the percentage of genes that significantly differentially expressed with Benjamini-Hochberg adjusted p-values less than 0.05, varies between 65%–80% (Figure 2, left panel). Approximately 33% of genes are differentially expressed across all four datasets and 20% of genes are differentially expressed in the same direction across all datasets. We also see clear cases where genes are consistently differentially expressed, but in different directions, where the overall p-values do not correlate with the absolute values of the sum of such genes’ ranked expression between subtypes (Figure 2, right panel, red points). We keep these genes to avoid introducing bias into the candidate gene lists.

Then, we enumerate all possible gene pairs from this reduced gene list. A small percent of these pairs has one gene express higher or lower than the other in all samples, resulting TSPs that are always 0 or 1 (Figure 3). To avoid collinearity with the intercept term in our model, we filter out these TSPs. We also remove TSPs with values equal to 0 or 1 in less than 10% samples in at least one study.

Next, we rank the TSPs by their likelihood in a marginal GLMM, assuming a study-level random slope and a random intercept. Our original approach removes lower ranked TSPs that share one same gene with higher ranked TSPs. Here we relax to only remove lower ranked TSPs if their absolute correlation coefficients with any higher ranked ones sharing one same gene is greater than 0.25.

Finally, we comment that users may set their own thresholds to cut the p-values and the correlation coefficients among TSPs. In our numerical work, we find that the prediction

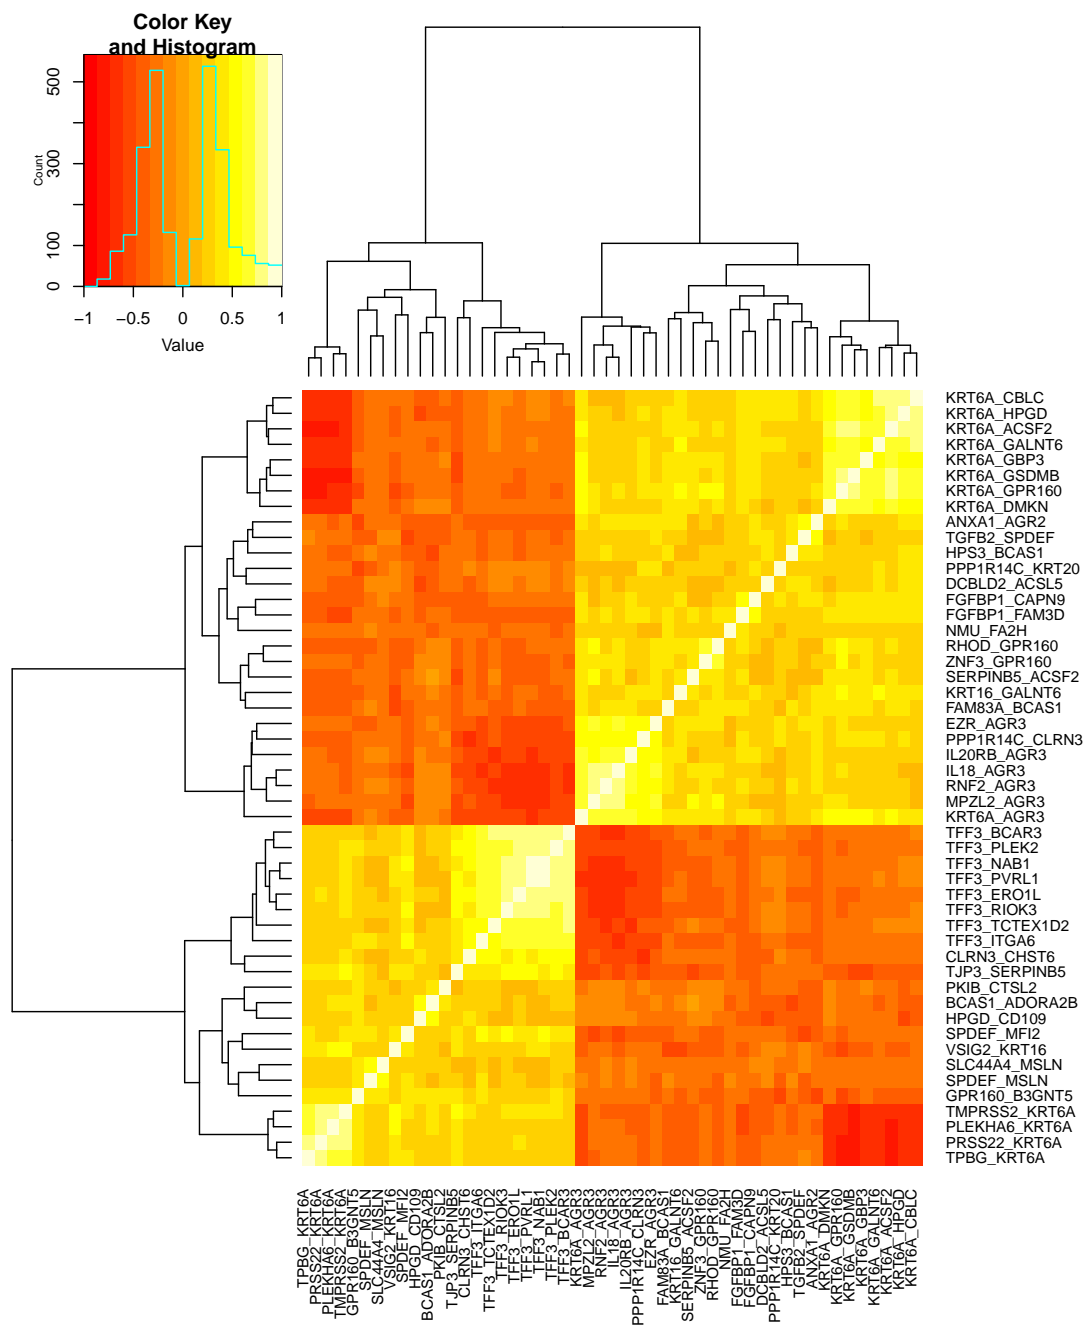

Figure 1: Correlation coefficients of the top 50 gene pairs rendered by the original screening.

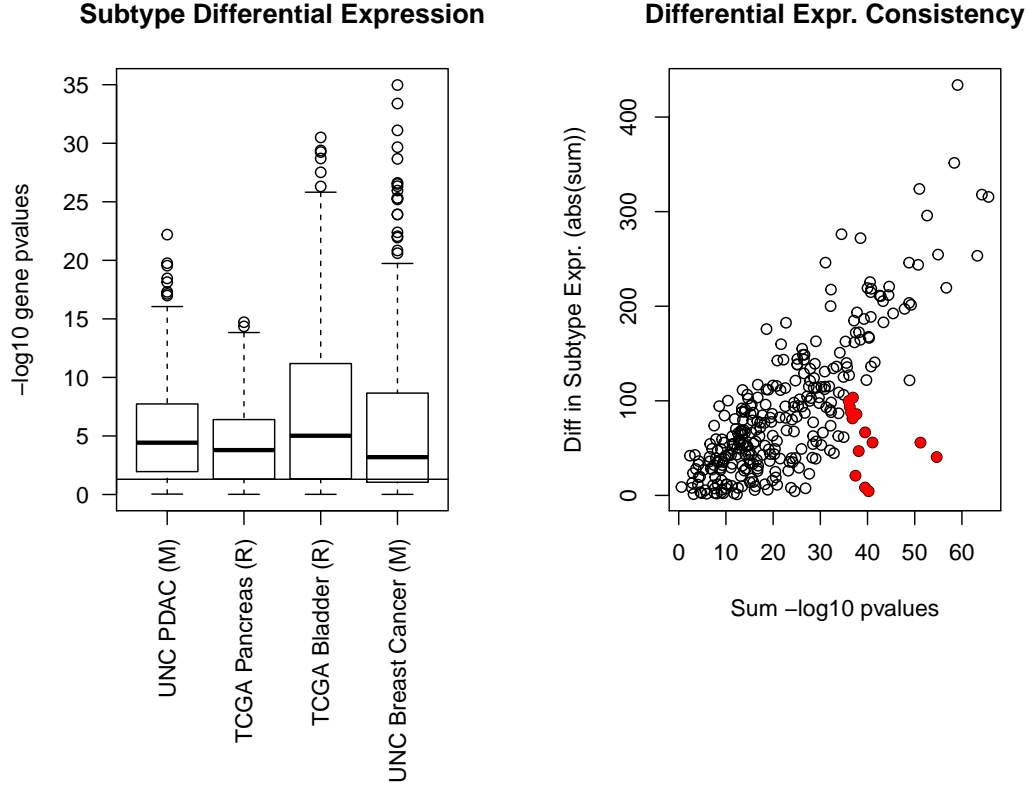

Figure 2: The Wilcoxon Rank Sum Test for testing differentially expressed genes. The left panel gives the boxplot of  $-\log_{10}(\text{p-values})$  for testing differential expression for every gene in each study. The right panel shows whether a gene is differentially expressed in the same direction in different studies. The absolute differences of a gene's expression rank in the two subtypes are summed across studies and plotted against its sum of  $-\log_{10}(\text{p-value})$  from all studies. Red dots represent genes that are differentially expressed in different directions across studies.

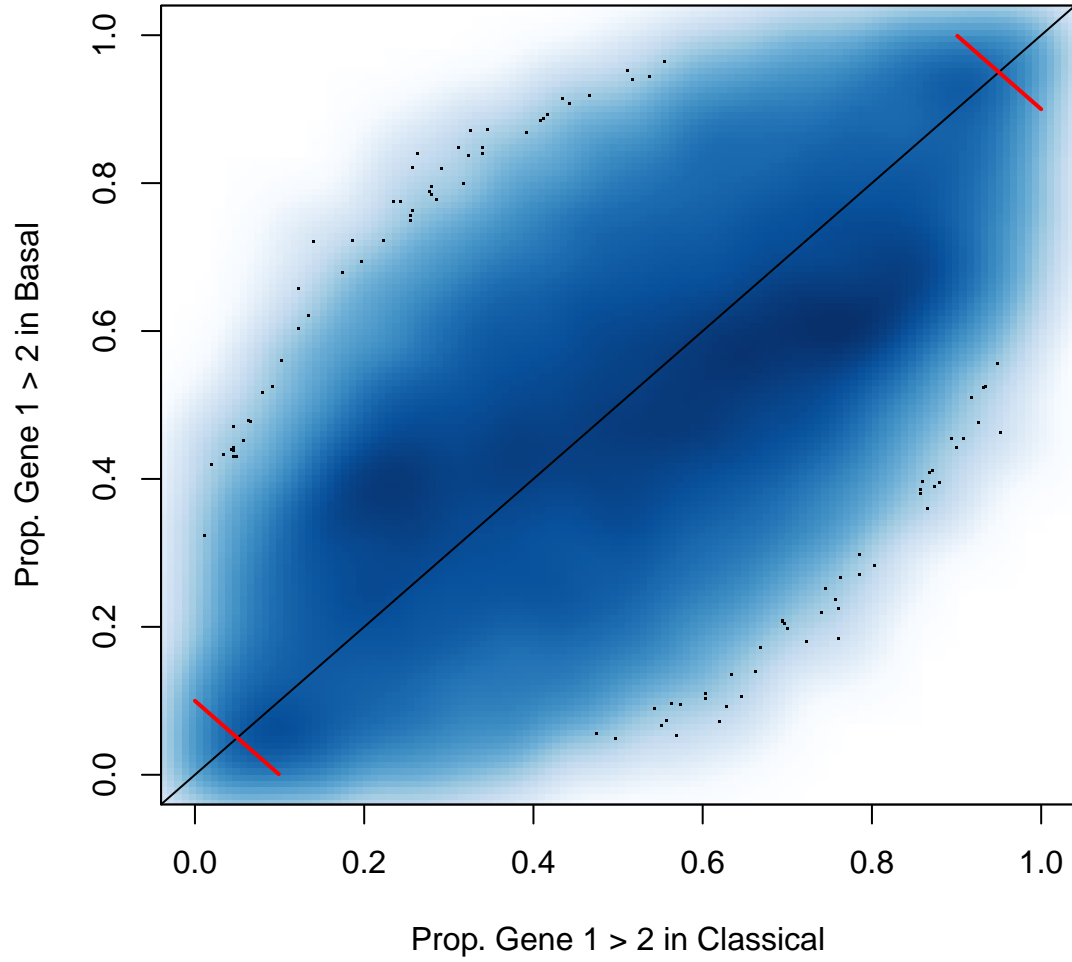

Figure 3: Percentages of gene pairs that have gene 1 express higher than gene 2 in the two subtypes. Red lines are boundaries where the resulting TSPs equal to 0 or 1 in less than 10% samples, beyond which the TSPs are filtered out.

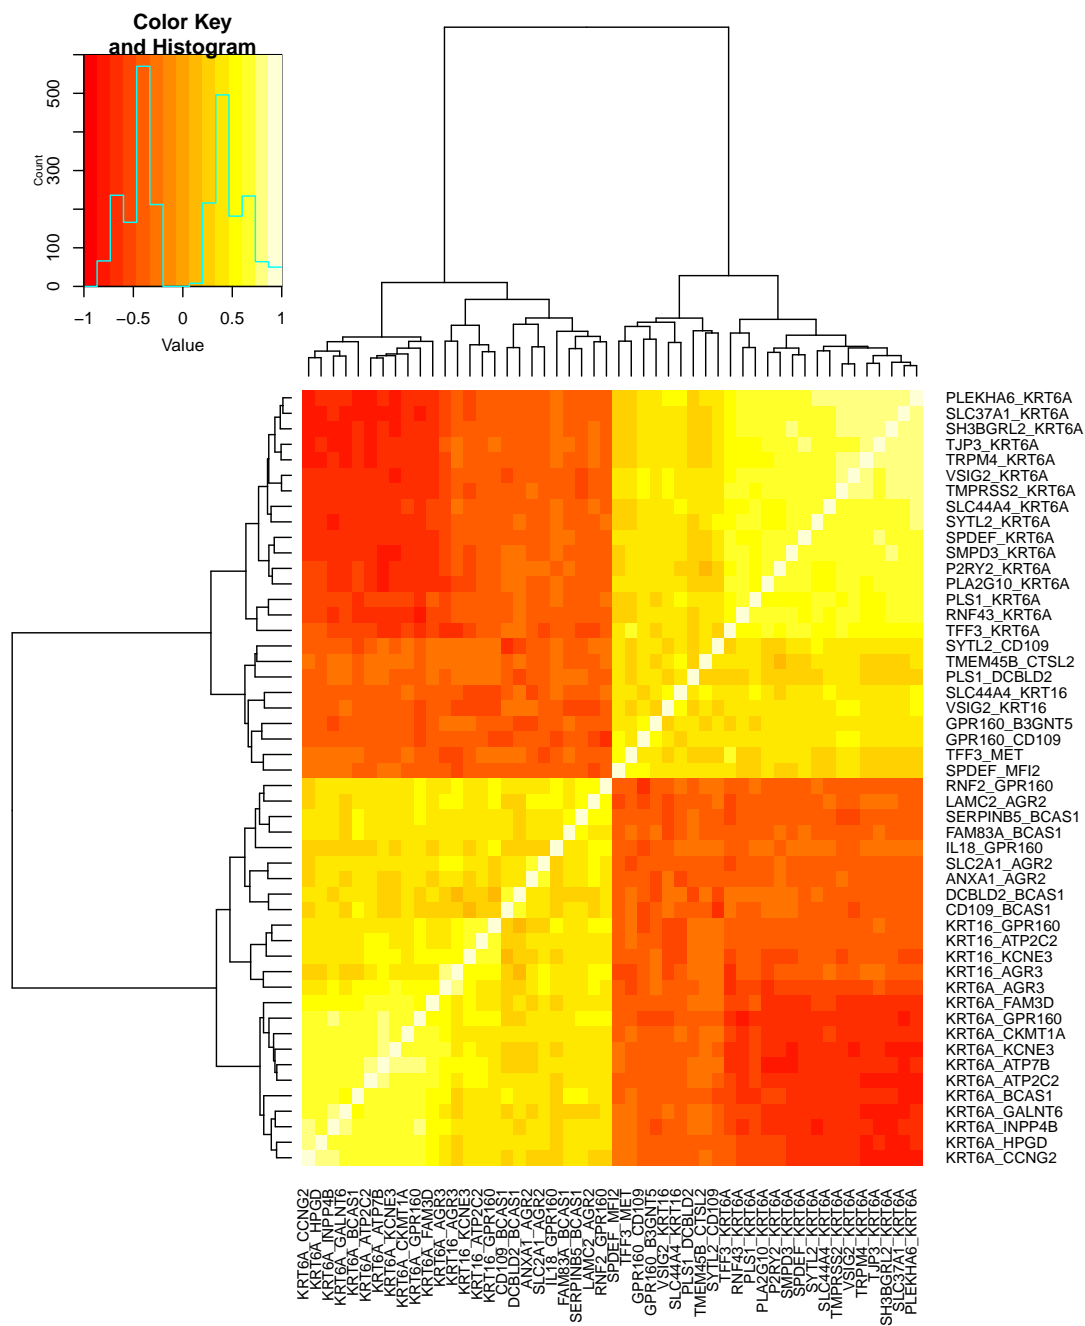

Figure 4: Correlation coefficients of the top 50 gene pairs rendered by the new screening.

error of our method is not very sensitive to such thresholds. A summary of the proposed screening steps is given as follows.

1. Take top 75% DE genes from the original gene list by their overall p-values across studies.
2. Enumerate all gene pairs to generate TSPs, remove those that equal to 0 or 1 in less than 10% samples in at least one study.
3. Rank TSPs by their likelihood in a marginal GLMM.
4. Remove lower ranked TSPs that are have absolute correlation coefficients  $> 0.25$  with higher ranked TSPs sharing one same gene.

In contrast to this, our previous screening approach is equivalent to setting the correlation threshold to equal to 0 in Item 4 above, effectively removing all lower gene pairs that have genes appearing in high ranked TSPs. We also did not apply Item 1 in our previous screening approach, instead filtering out TSPs with TSP score (as defined by the `tspair` package) less than 0.4.

## **S2 Additional analysis results of the PDAC data**

The new screening approach in the prior section yields 107 TSPs, based on which we repeat the same analysis as in the main manuscript. The results are summarized in Figures 5–7. We find that our pGLMMC method still has small prediction errors (PE), albeit only a slight improvement in terms of median overall PE compared to the pGLMC. Compared to the results in the main manuscript, the prediction errors remain at similar levels for the pGLMMC. Under the new screening, the pGLMMC selects fewer number of predictors to have non-zero variance across datasets. As a result, the improvement of the pGLMMC over the pGLMC is not as pronounced as shown in the main manuscript. The pGLM and the Meta-Lasso remain to have large prediction errors.

Using the TSPs from the new screening, we also perform a holdout prediction study across platforms. More specifically, we combine microarray data (studies 1 and 4), apply

the pGLMMC to fit a model, use the resulting model to predict subtypes from RNA-seq platforms (studies 2 and 3), and vice versa. The boxplots of absolute prediction errors are given in Figure 8. It is seen that the prediction errors are similar to the original holdout study, which suggests that platform may not severely impact our method’s prediction performance.



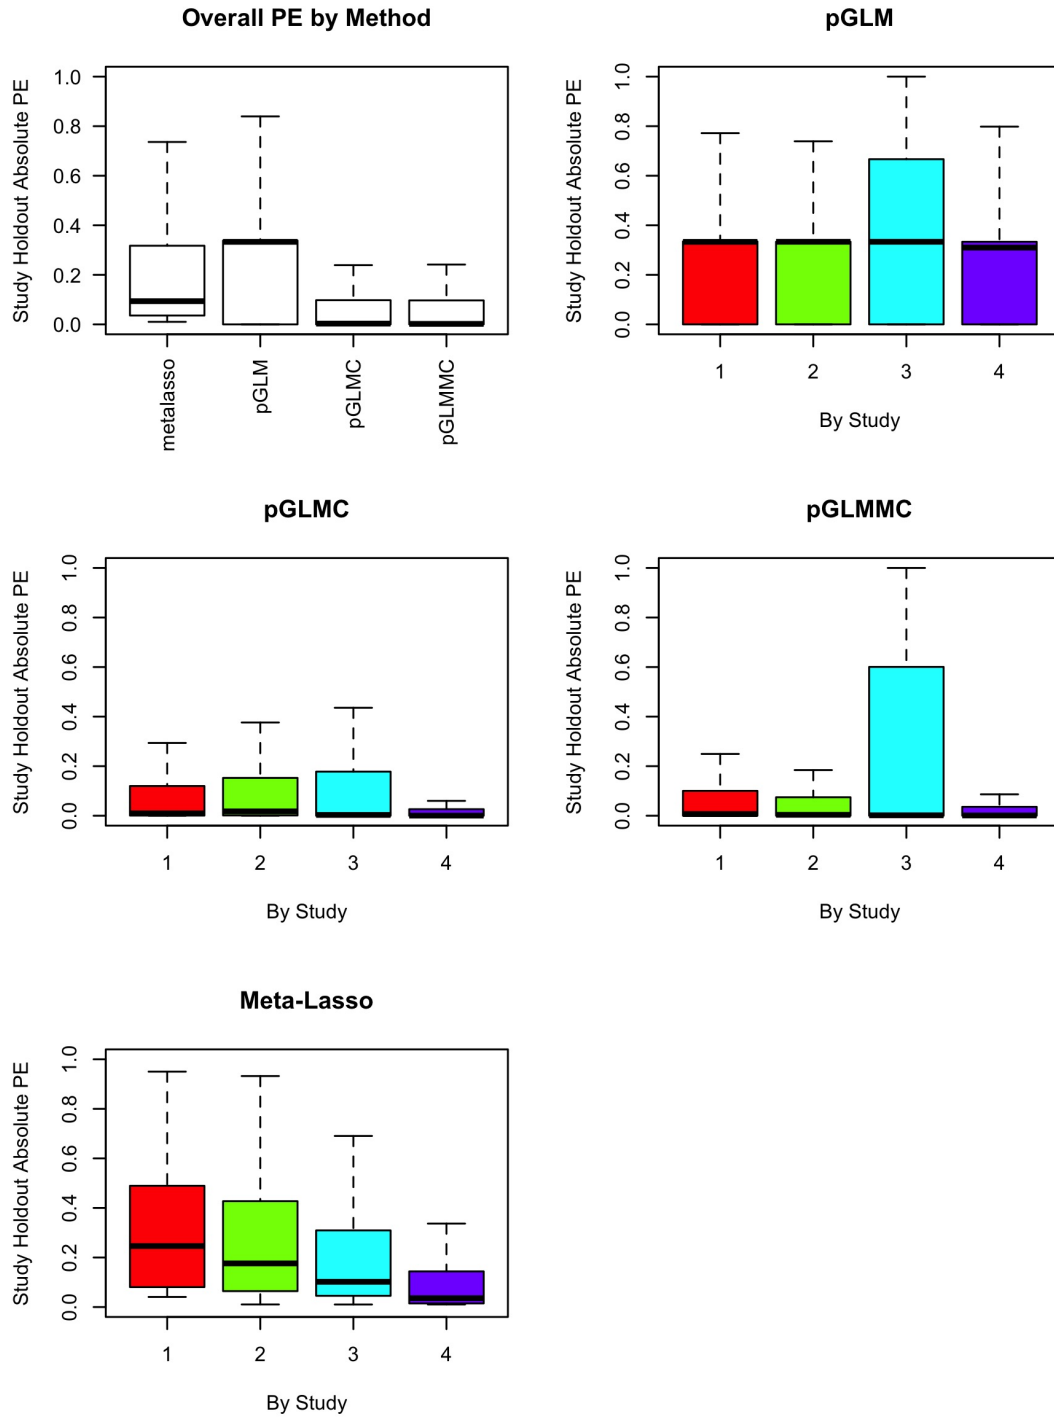

Figure 6: Prediction errors of the holdout studies given by the four methods.

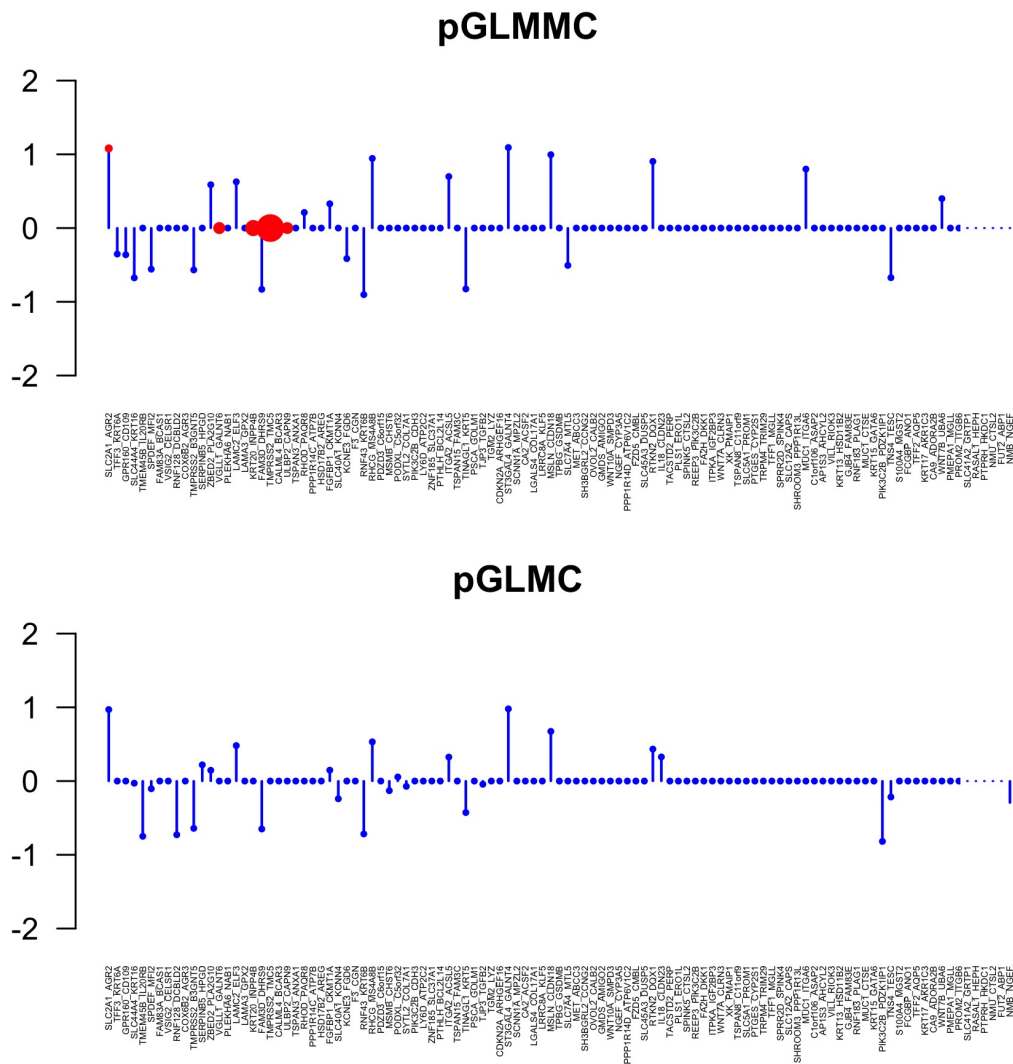

Figure 7: Estimated coefficients given by the pGLMC and the pGLMMC. Red circles indicate variables with non-zero random effects estimated by the pGLMMC. Larger red dots indicate larger estimated between-study variance.

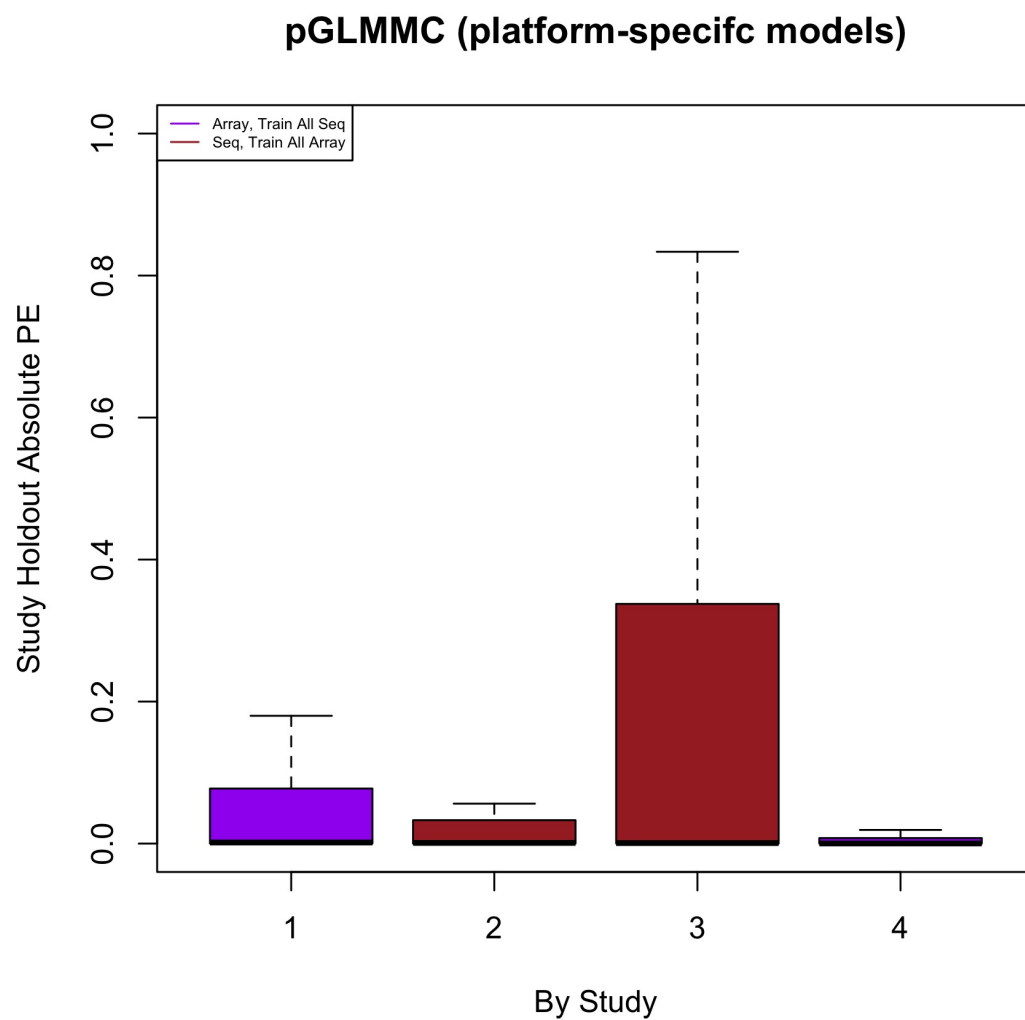

Figure 8: Prediction errors by the pGLMMC trained on a different platform. Red denotes RNA-seq data and purple denotes microarray data.

### S3 Proofs

We need the following conditions to establish the theoretical properties in Section 5.

- (C1)  $b(\vartheta)$  is twice continuously differentiable.
- (C2) For all  $1 \leq k \leq K$  and  $1 \leq i \leq n$ , there exists a constant  $M$  such that  $\max_{1 \leq j \leq p} |x_{ki,j}| \leq M$ .
- (C3)  $s_n c_n = o(1)$ .
- (C4)  $s_n = o(n^\delta)$ ,  $b_n \gg n^{-\delta}$ ,  $s_n^{3/2} b_n = o(n^{1/2-\delta})$ , and  $\log d_n = o(n)$ .
- (C5)  $\|\{E[\nabla_{\boldsymbol{\theta}_s}^2 \ell(\boldsymbol{\theta}^*)]\}^{-1}\|_\infty = O(1)$ .
- (C6)  $\|\{E[\nabla_{\boldsymbol{\theta}_{sc}} \ell(\boldsymbol{\theta}^*)]\} \{E[\nabla_{\boldsymbol{\theta}_s}^2 \ell(\boldsymbol{\theta}^*)]\}^{-1}\|_\infty < \min\{\frac{\rho'(0+)}{\rho'(b_n)}, Ln^\xi\}$  for some  $L > 0$  and  $0 < \xi < 1/2$ .
- (C7)  $\sup_{\boldsymbol{\theta} \in \mathcal{N}} \max_{1 \leq j \leq s_n} \|\nabla_{\boldsymbol{\theta}_s}^2 \{E[\nabla_{\boldsymbol{\theta}} \ell(\boldsymbol{\theta})]\}_j\|_2 = O(1)$ .
- (C8)  $\rho(t)$  is increasing and concave in  $t \in [0, \infty)$  and has a continuous derivative  $\rho'(t)$  with  $\rho'(0+) > 0$ .

Conditions (C1) and (C2) are standard conditions for the GLMM. Conditions (C3) and (C4) are sparsity conditions on  $s_n$  and conditions required for the minimal signal of  $b_n$ . These conditions require  $s_n \ll n$  and  $b_n$  to be bounded away from 0. Conditions (C5)-(C7) are common conditions for establishing variable selection consistency (Fan and Lv, 2011). Due to the usage of the folded-concave penalty, the upper bound in (C6) is allowed to grow at an order of  $n^\xi$  for  $0 < \xi < 1/2$ . Condition (C8) defines the class of folded-concave penalty functions.

To prove Theorem 1, we first provide a maximal inequality for the gradient  $\nabla_{\boldsymbol{\theta}_j} \ell(\boldsymbol{\theta})$  when  $\boldsymbol{\theta}$  varies in the neighborhood  $\mathcal{N}$ .

**Lemma 1.** *Under conditions (C1)–(C3), it holds that*

$$P\left(\left|\sup_{\boldsymbol{\theta} \in \mathcal{N}} \left\{\nabla_{\boldsymbol{\theta}_j} \ell(\boldsymbol{\theta}) - E[\nabla_{\boldsymbol{\theta}_j} \ell(\boldsymbol{\theta})]\right\}\right| > C_1 s_n^{3/2} b_n / n^{1/2} + C_2 t\right) \leq K \exp(-C_3 n t^2),$$

where  $C_1$ ,  $C_2$  and  $C_3$  are some universal positive constants.

**Proof of Lemma 1.** Let  $\ell_k(\boldsymbol{\theta})$  be the log-likelihood of the  $k$ -th dataset (after removing constants that do not depend on  $\boldsymbol{\theta}$ ), which is given by

$$\ell_k(\boldsymbol{\theta}) = \frac{1}{n} \sum_{i=1}^n \log \int_{\mathcal{R}^{q_n}} \exp\{y_{ki} \vartheta_{ki} - b(\vartheta_{ki})\} \phi(\boldsymbol{\alpha}_k) d\boldsymbol{\alpha}_k.$$

Define

$$U_{1kj}(\boldsymbol{\theta}) = \nabla_{\beta_j} \ell_k(\boldsymbol{\theta}) = \frac{\int_{\mathcal{R}^{q_n}} \{y_{ki} - b'(\vartheta_{ki})\} \exp\{y_{ki}\vartheta_{ki} - b(\vartheta_{ki})\} x_{ki,j} \phi(\boldsymbol{\alpha}_k) d\boldsymbol{\alpha}_k}{\int_{\mathcal{R}^{q_n}} \exp\{y_{ki}\vartheta_{ki} - b(\vartheta_{ki})\} \phi(\boldsymbol{\alpha}_k) d\boldsymbol{\alpha}_k} \quad (\text{S.1})$$

$$U_{2kj}(\boldsymbol{\theta}) = \nabla_{\gamma_{t_j}} \ell_k(\boldsymbol{\theta}) = \frac{\int_{\mathcal{R}^{q_n}} \{y_{ki} - b'(\vartheta_{ki})\} \exp\{y_{ki}\vartheta_{ki} - b(\vartheta_{ki})\} \mathbf{z}_{ki}^T \text{mat}(\mathbf{J}_{q_n, t_j}) \boldsymbol{\alpha}_k \phi(\boldsymbol{\alpha}_k) d\boldsymbol{\alpha}_k}{\int_{\mathcal{R}^{q_n}} \exp\{y_{ki}\vartheta_{ki} - b(\vartheta_{ki})\} \phi(\boldsymbol{\alpha}_k) d\boldsymbol{\alpha}_k}, \quad (\text{S.2})$$

where  $\mathbf{J}_{q_n, t_j}$  is the  $t_j$ -th column of  $\mathbf{J}_{q_n}$ , and  $\text{mat}(\cdot)$  is an operator that transforms the vector into a  $q_n \times q_n$  matrix. Observe that only one element in  $\text{mat}(\mathbf{J}_{q_n, t_j})$  is one and all others are zero. Let

$$\begin{aligned} S_{1kj}(\boldsymbol{\theta}) &= \frac{1}{n} \sum_{i=1}^n U_{1kj}(\boldsymbol{\theta}), & s_{1kj}(\boldsymbol{\theta}) &= \mathbb{E}[U_{1kj}(\boldsymbol{\theta})]; \\ S_{2kj}(\boldsymbol{\theta}) &= \frac{1}{n} \sum_{i=1}^n U_{2kj}(\boldsymbol{\theta}), & s_{2kj}(\boldsymbol{\theta}) &= \mathbb{E}[U_{2kj}(\boldsymbol{\theta})]. \end{aligned}$$

First, we show that, for any  $1 \leq k \leq K$ ,  $1 \leq j \leq p_n$ , there exist positive constants  $C_1, C_2, C_3$  such that

$$P \left( \sup_{\boldsymbol{\theta} \in \mathcal{N}} |S_{1kj}(\boldsymbol{\theta}) - s_{1kj}(\boldsymbol{\theta})| \geq C_1 s_n^{3/2} b_n / n^{1/2} + C_2 t \right) \leq \exp(-C_3 n t^2); \quad (\text{S.3})$$

$$P \left( \sup_{\boldsymbol{\theta} \in \mathcal{N}} |S_{2kj}(\boldsymbol{\theta}) - s_{2kj}(\boldsymbol{\theta})| \geq C_1 s_n^{3/2} b_n / n^{1/2} + C_2 t \right) \leq \exp(-C_3 n t^2). \quad (\text{S.4})$$

To prove (S.3), we define the class of functions  $\mathcal{F} = \{U_{1kj}(\boldsymbol{\theta}) : \boldsymbol{\theta} \in \mathcal{N}\}$ . We first calculate the bracketing entropy of  $\mathcal{F}$ . For any  $\boldsymbol{\theta}_1 = (\boldsymbol{\beta}_1, \boldsymbol{\gamma}_1)^T \in \mathcal{N}$  and  $\boldsymbol{\theta}_2 = (\boldsymbol{\beta}_2, \boldsymbol{\gamma}_2)^T \in \mathcal{N}$ , define  $\vartheta_{k1} = \mathbf{x}_k^T \boldsymbol{\beta}_1 + (\boldsymbol{\alpha}_k \otimes \mathbf{z}_k)^T \mathbf{J}_{q_n} \boldsymbol{\gamma}_1$  and  $\vartheta_{k2} = \mathbf{x}_k^T \boldsymbol{\beta}_2 + (\boldsymbol{\alpha}_k \otimes \mathbf{z}_k)^T \mathbf{J}_{q_n} \boldsymbol{\gamma}_2$ . We have

$$\begin{aligned} |U_{1kj}(\boldsymbol{\theta}_1) - U_{1kj}(\boldsymbol{\theta}_2)| &= |U'_{1kj}(\tilde{\boldsymbol{\theta}})| |\vartheta_{k1} - \vartheta_{k2}| \\ &\stackrel{(i)}{\lesssim} |\mathbf{x}_k^T (\boldsymbol{\beta}_1 - \boldsymbol{\beta}_2) + (\boldsymbol{\alpha}_k \otimes \mathbf{z}_k)^T \mathbf{J}_{q_n} (\boldsymbol{\gamma}_1 - \boldsymbol{\gamma}_2)| \\ &\leq s_{1n} \|\boldsymbol{\beta}_1 - \boldsymbol{\beta}_2\|_\infty + s_{2n} \|\boldsymbol{\gamma}_1 - \boldsymbol{\gamma}_2\|_\infty \\ &\leq s_n \|\boldsymbol{\theta}_1 - \boldsymbol{\theta}_2\|_\infty, \end{aligned}$$

where  $\tilde{\boldsymbol{\theta}}$  is a vector lying on the line segment connecting  $\boldsymbol{\theta}_1$  and  $\boldsymbol{\theta}_2$ . In (i), the smoothness condition (C1) implies that  $U'_{1kj}(\boldsymbol{\theta})$  is continuous. Hence,  $\sup_{\boldsymbol{\theta} \in \mathcal{N}} |U'_{1kj}(\boldsymbol{\theta})|$  is bounded by a constant  $M$ . Therefore, the bracketing entropy of  $\mathcal{F}$  is at most of the order  $s_n \log(M s_n b_n / \epsilon)$

(see Example 19.7 of Van der Vaart (2000)). Then, for the entropy integral, we have

$$\int_0^1 \sqrt{s_n \log(M s_n b_n / \epsilon)} d\epsilon \lesssim s_n^{3/2} b_n.$$

Next, for the purposes of applying the maximal inequality, we show that for any  $1 \leq k \leq K$ ,  $1 \leq j \leq p_n$  and  $\boldsymbol{\theta} \in \mathcal{N}$ , there exists uniform positive constants  $\sigma$  and  $c$  such that, for all integers  $l \geq 2$ ,

$$\mathbb{E}|U_{1kj}(\boldsymbol{\theta})|^l \leq \frac{l!}{2} \sigma^2 c^{l-2} \quad \text{and} \quad \mathbb{E}|U_{2kj}(\boldsymbol{\theta})|^l \leq \frac{l!}{2} \sigma^2 c^{l-2}.$$

In other words, the gradients  $U_{1kj}(\boldsymbol{\theta})$  and  $U_{2kj}(\boldsymbol{\theta})$  have exponential tails. Note that  $U_{1kj}(\boldsymbol{\theta}) = I_1(\boldsymbol{\theta}) + I_2(\boldsymbol{\theta})$ , where

$$\begin{aligned} I_1(\boldsymbol{\theta}) &= \frac{\int_{\mathcal{R}^{q_n}} \{y_{ki} - b'(\vartheta_{ki}^*)\} \exp\{y_{ki}\vartheta_{ki} - b(\vartheta_{ki})\} x_{ki,j} \phi(\boldsymbol{\alpha}_k) d\boldsymbol{\alpha}_k}{\int_{\mathcal{R}^{q_n}} \exp\{y_{ki}\vartheta_{ki} - b(\vartheta_{ki})\} \phi(\boldsymbol{\alpha}_k) d\boldsymbol{\alpha}_k}, \\ I_2(\boldsymbol{\theta}) &= \frac{\int_{\mathcal{R}^{q_n}} \{b'(\vartheta_{ki}^*) - b'(\vartheta_{ki})\} \exp\{y_{ki}\vartheta_{ki} - b(\vartheta_{ki})\} x_{ki,j} \phi(\boldsymbol{\alpha}_k) d\boldsymbol{\alpha}_k}{\int_{\mathcal{R}^{q_n}} \exp\{y_{ki}\vartheta_{ki} - b(\vartheta_{ki})\} \phi(\boldsymbol{\alpha}_k) d\boldsymbol{\alpha}_k}. \end{aligned}$$

Since the distribution of  $y_{ki}$  belongs to the exponential family, there exists positive constants  $\sigma_0$  and  $c_0$  such that  $\mathbb{E}|y_{ki}|^l \leq l! \sigma_0^2 c_0^{l-2} / 2$ . By conditions (C1) and (C2),  $x_{ki,j}$  and  $b'(\vartheta_{ki}^*)$  are bounded. Using Hölder's inequality, we have  $\mathbb{E}|I_1(\boldsymbol{\theta})|^l \leq l! \sigma_1^2 c_1^{l-2} / 2$  for some constants  $\sigma_1$  and  $c_1$ . On the other hand,

$$\begin{aligned} |I_2(\boldsymbol{\theta})|^l &\lesssim \left\{ \sup_{\boldsymbol{\theta} \in \mathcal{N}} |b'(\vartheta_{ki}^*) - b'(\vartheta_{ki})| \right\}^l \lesssim \left\{ \sup_{\boldsymbol{\theta} \in \mathcal{N}} |\vartheta_{ki}^* - \vartheta_{ki}| \right\}^l \\ &\lesssim \left\{ \sup_{\boldsymbol{\theta} \in \mathcal{N}} |\mathbf{x}_{ki}^T (\boldsymbol{\beta}^* - \boldsymbol{\beta}) + (\mathbf{z}_{ki} \otimes \boldsymbol{\alpha}_{ki})^T \mathbf{J}_{q_n} (\boldsymbol{\gamma}^* - \boldsymbol{\gamma})| \right\}^l \\ &\lesssim s_n \sup_{\boldsymbol{\theta} \in \mathcal{N}} \|\boldsymbol{\theta} - \boldsymbol{\theta}^*\|_\infty = O(s_n c_n) = o(1), \end{aligned}$$

Therefore, there exists positive constants  $\sigma$  and  $c$  such that  $\mathbb{E}|U_{1kj}(\boldsymbol{\theta})|^l \leq (l!/2) \sigma^2 c^{l-2}$ . A similar result can be shown for  $U_{2kj}(\boldsymbol{\theta})$ .

Applying the maximal inequality (Massart, 2007), for any  $x > 0$ , there exists constants  $A_1$  and  $A_2$  such that

$$P \left( \sup_{\boldsymbol{\theta} \in \mathcal{N}} |S_{1kj}(\boldsymbol{\theta}) - s_{1kj}(\boldsymbol{\theta})| \geq C_1 s_n^{3/2} b_n / n^{1/2} + A_1 \sqrt{x/n} + A_2 x/n \right) \leq \exp(-x).$$

Let  $t = \sqrt{x/n}$ . Then, for any  $t \leq A_1 A_2^{-1}$ ,  $A_1 \sqrt{x/n} \geq A_2 x/n$ . Hence,  $A_1 \sqrt{x/n} + A_2 x/n \leq C_2 \sqrt{x/n}$ , where  $C_2 = 2A_1$ . Therefore,

$$P \left( \sup_{\boldsymbol{\theta} \in \mathcal{N}} |S_{1kj}(\boldsymbol{\theta}) - s_{1kj}(\boldsymbol{\theta})| \geq C_1 s_n^{3/2} b_n / n^{1/2} + C_2 t \right) \leq \exp(-C_3 n t^2).$$

This completes the proof of (S.3).

Finally, notice that the gradient of  $\ell(\boldsymbol{\theta})$  is given by

$$\nabla_{\beta_j} \ell(\boldsymbol{\theta}) = \sum_{k=1}^K S_{1kj}(\boldsymbol{\theta}) \quad \text{and} \quad \nabla_{\gamma_{t_j}} \ell(\boldsymbol{\theta}) = \sum_{k=1}^K S_{2kj}(\boldsymbol{\theta}).$$

Then, it follows from (S.3), (S.4) and the union bound that the result holds.  $\square$

**Proof of Theorem 1.** By Karush–Kuhn–Tucker conditions, any vector  $\widehat{\boldsymbol{\theta}}$  satisfying (S.5)–(S.9) is a solution to 4, and

$$\nabla_{\beta_j} \ell(\widehat{\boldsymbol{\theta}}) = \lambda_1 \rho'(|\widehat{\beta}_j|) \text{sgn}(\widehat{\beta}_j), \text{ for } \widehat{\beta}_j \neq 0; \quad (\text{S.5})$$

$$\nabla_{\gamma_t} \ell(\widehat{\boldsymbol{\theta}}) = \lambda_2 \rho'(\|\widehat{\gamma}_t\|_2) \frac{\widehat{\gamma}_t}{\|\widehat{\gamma}_t\|_2}, \text{ for } \widehat{\gamma}_t \neq \mathbf{0}; \quad (\text{S.6})$$

$$\left| \left[ \nabla_{\beta_j} \ell(\widehat{\boldsymbol{\theta}}) \right]_{\widehat{\beta}_j=0} \right| < \lambda_1 \rho'(0+), \text{ for } \widehat{\beta}_j = 0; \quad (\text{S.7})$$

$$\left\| \left[ \nabla_{\gamma_t} \ell(\widehat{\boldsymbol{\theta}}) \right]_{\widehat{\gamma}_t=\mathbf{0}} \right\|_2 < \lambda_2 \rho'(0+), \text{ for } \widehat{\gamma}_t = \mathbf{0}; \quad (\text{S.8})$$

$$\lambda_{\min} \left( \nabla_{\boldsymbol{\theta}_S}^2 \ell(\widehat{\boldsymbol{\theta}}) \right) > (\lambda_1 + \lambda_2) \kappa(\rho, \mathbf{u}), \quad (\text{S.9})$$

where the sign function is defined as  $\text{sgn}(x) = 1$  for  $x > 0$  and  $\text{sgn}(x) = -1$  for  $x < 0$ .

Let  $\boldsymbol{\eta} = \nabla_{\boldsymbol{\theta}} \ell(\boldsymbol{\theta}) - \mathbb{E}[\nabla_{\boldsymbol{\theta}} \ell(\boldsymbol{\theta})]$  and  $A = A_1 \cap A_2$ , where

$$A_1 = \left\{ \left\| \sup_{\boldsymbol{\theta} \in \mathcal{N}} \boldsymbol{\eta}_S \right\|_{\infty} \leq C_1 s_n^{3/2} b_n / \sqrt{n} + D \sqrt{(\log d_n)/n} \right\},$$

$$A_2 = \left\{ \left\| \sup_{\boldsymbol{\theta} \in \mathcal{N}} \boldsymbol{\eta}_{S^c} \right\|_{\infty} \leq C_1 s_n^{3/2} b_n / \sqrt{n} + D \sqrt{(\log d_n)/n} \right\},$$

for a sufficiently large constant  $D$ . Lemma 1 together with the union bound imply that

$$P(A_2 \cap A_2) \geq 1 - P(A_1^c) - P(A_2^c) \geq 1 - \{K s_n n^{-C} + K(d_n - s_n) d_n^{-C}\}. \quad (\text{S.10})$$

For the event  $A_1 \cap A_2$ , we show that the following two results hold. They together with (S.10) complete the proof.

- [1] Within the hypercube  $\mathcal{C} = \{\boldsymbol{\theta}_S : \|\boldsymbol{\theta}_S - \boldsymbol{\theta}_S^*\|_{\infty} \leq c n^{-\delta}\}$ , where  $c$  is a positive constant, there exists a vector  $\widehat{\boldsymbol{\theta}}_S$  satisfying (S.5), (S.6), and (S.9).
- [2] The vector  $\widehat{\boldsymbol{\theta}} = (\widehat{\boldsymbol{\theta}}_S, \mathbf{0})^T$  also satisfies (S.7) and (S.8).

To show statement [1], denote the  $s_n \times 1$  vector

$$\boldsymbol{\tau}_S = \left( \lambda_1 K \rho'(|\beta_j|) \text{sgn}(\beta_j), \lambda_2 K \rho'(\|\gamma_t\|_2) \frac{\gamma_t}{\|\gamma_t\|_2} \right)^T \text{ for } j \in S_1 \text{ and } t \in S_2.$$

Since  $\mathbb{E}[\nabla_{\boldsymbol{\theta}} \ell(\boldsymbol{\theta}^*)] = \mathbf{0}$ , by a Taylor's series expansion, we have

$$\nabla_{\boldsymbol{\theta}_S} \ell(\boldsymbol{\theta}) = \mathbb{E}[\nabla_{\boldsymbol{\theta}_S} \ell(\boldsymbol{\theta})] - \mathbb{E}[\nabla_{\boldsymbol{\theta}_S} \ell(\boldsymbol{\theta}^*)] + \boldsymbol{\eta}_S = \mathbb{E}[\nabla_{\boldsymbol{\theta}_S}^2 \ell(\boldsymbol{\theta}^*)](\boldsymbol{\theta}_S - \boldsymbol{\theta}_S^*) + \mathbf{r}_S + \boldsymbol{\eta}_S,$$

where  $\mathbf{r}_S$  is an  $s_n \times 1$  vector such that its  $j$ -th element equals to  $(\boldsymbol{\theta}_S - \boldsymbol{\theta}_S^*)^T \nabla_{\boldsymbol{\theta}_S}^2 \{\mathbb{E}[\nabla_{\boldsymbol{\theta}_S} \ell(\bar{\boldsymbol{\theta}})]\}_j (\boldsymbol{\theta}_S - \boldsymbol{\theta}_S^*)$ , and  $\bar{\boldsymbol{\theta}}$  is a vector lying on the line segment joining  $\boldsymbol{\theta}$  and  $\boldsymbol{\theta}^*$ . By condition (C7),

$$\|\mathbf{r}_S\|_{\infty} = O(\|\boldsymbol{\theta}_S - \boldsymbol{\theta}_S^*\|_2) = O(s_n n^{-2\delta}). \quad (\text{S.11})$$

Since  $b_n \gg n^{-\delta}$ , for any  $\boldsymbol{\theta}_S \in \mathcal{C}$ , we have for its  $j$ -th element that

$$\min_{1 \leq j \leq s_n} |\theta_{S,j}| \geq \min_{1 \leq j \leq s_n} |\theta_{S,j}^*| - b_n \geq b_n.$$

By condition (C8),  $\rho'(t)$  is a decreasing function for  $t \in [0, \infty)$ . Hence,  $\rho'(|\theta_{S,j}|) \leq \rho'(b_n)$ .

Therefore,

$$\begin{aligned} \lambda_1 \rho'(|\hat{\beta}_j|) |\text{sgn}(\hat{\beta}_j)| &\leq \lambda_1 \rho'(b_n), \text{ for all } j \in S_1, \\ \lambda_2 \rho'(\|\hat{\gamma}_t\|_2) \|\hat{\gamma}_t\|_2^{-1} \|\hat{\gamma}_t\|_{\infty} &\leq \lambda_2 \rho'(b_n), \text{ for all } t \in S_2. \end{aligned}$$

Hence,

$$\|\boldsymbol{\tau}_S\|_{\infty} = O(\lambda_{un} \rho'(b_n)). \quad (\text{S.12})$$

Then, by condition (C5), (S.11), (S.12) and the stated choice of  $\lambda_1$  and  $\lambda_2$ , we have

$$\begin{aligned} \|\{\mathbb{E}[\nabla_{\boldsymbol{\theta}_S}^2 \ell(\boldsymbol{\theta}^*)]\}^{-1}(\mathbf{r}_S + \boldsymbol{\eta}_S + \boldsymbol{\tau}_S)\|_{\infty} &\leq \|\{\mathbb{E}[\nabla_{\boldsymbol{\theta}_S}^2 \ell(\boldsymbol{\theta}^*)]\}^{-1}\|_{\infty} (\|\mathbf{r}_S\|_{\infty} + \|\boldsymbol{\eta}_S\|_{\infty} + \|\boldsymbol{\tau}_S\|_{\infty}) \\ &= O(s_n n^{-2\delta} + s_n^{3/2} b_n / \sqrt{n} + \sqrt{(\log d_n)/n} + 2\lambda_{un} \rho'(b_n)) \\ &= o(n^{-\delta}). \end{aligned}$$

Define  $\mathbf{f}(\boldsymbol{\theta}_S) = \mathbb{E}[\nabla_{\boldsymbol{\theta}_S}^2 \ell(\boldsymbol{\theta}^*)](\boldsymbol{\theta}_S - \boldsymbol{\theta}_S^*) + \mathbf{r}_S + \boldsymbol{\eta}_S - \boldsymbol{\tau}_S$  and  $\mathbf{g}(\boldsymbol{\theta}_S) = \{\mathbb{E}[\nabla_{\boldsymbol{\theta}_S}^2 \ell(\boldsymbol{\theta}^*)]\}^{-1} \mathbf{f}(\boldsymbol{\theta}_S)$ .

For sufficiently large  $n$ , if  $|\theta_j - \theta_j^*| = n^{-\delta}$ ,

$$\{\mathbf{g}(\boldsymbol{\theta}_S)\}_j \geq n^{-\delta} - \|\{\mathbb{E}[\nabla_{\boldsymbol{\theta}_S}^2 \ell(\boldsymbol{\theta})]\}^{-1}(\mathbf{r}_S + \boldsymbol{\eta}_S + \boldsymbol{\tau}_S)\|_{\infty} > 0.$$

If  $|\theta_j - \theta_j^*| = -n^{-\delta}$ ,  $\{\mathbf{g}(\boldsymbol{\theta})\}_j \leq -n^{-\delta} + \|\{\mathbb{E}[\nabla_{\boldsymbol{\theta}_S}^2 \ell(\boldsymbol{\theta})]\}^{-1}(\mathbf{r}_S + \boldsymbol{\eta}_S + \boldsymbol{\tau}_S)\|_{\infty} < 0$ . Since the function  $\mathbf{g}(\boldsymbol{\theta})$  is continuous in  $\mathcal{N}$ , an application of Miranda's existence theorem (Vrahatis, 1989) implies that the equation  $\mathbf{g}(\boldsymbol{\theta}) = \mathbf{0}$  has a solution  $\hat{\boldsymbol{\theta}}$  in  $\mathcal{C}$ . Hence,  $\hat{\boldsymbol{\theta}}$  also solves

$\mathbf{f}(\boldsymbol{\theta}) = \mathbf{0}$  and further solves (S.5) and (S.6). Finally, by the stated choices of  $\lambda_1$  and  $\lambda_2$ , (S.9) also holds for  $\widehat{\boldsymbol{\theta}}_S$ . This completes the proof of statement [1].

To show statement [2], by a Taylor's series expansion, we have

$$\begin{aligned}\nabla_{\boldsymbol{\theta}_{Sc}} \ell(\widehat{\boldsymbol{\theta}}) &= \mathbb{E}[\nabla_{\boldsymbol{\theta}_{Sc}} \ell(\widehat{\boldsymbol{\theta}})] - \mathbb{E}[\nabla_{\boldsymbol{\theta}_{Sc}} \ell(\boldsymbol{\theta}^*)] + \boldsymbol{\eta}_{Sc} \\ &= \mathbb{E}[\nabla_{\boldsymbol{\theta}_{Sc} \boldsymbol{\theta}_S} \ell(\boldsymbol{\theta}^*)](\widehat{\boldsymbol{\theta}}_S - \boldsymbol{\theta}_S^*) + \boldsymbol{\eta}_{Sc} + \mathbf{r}_{Sc} \\ &= \mathbb{E}[\nabla_{\boldsymbol{\theta}_{Sc} \boldsymbol{\theta}_S} \ell(\boldsymbol{\theta}^*)] \left\{ \mathbb{E}[\nabla_{\boldsymbol{\theta}_S}^2 \ell(\boldsymbol{\theta}^*)] \right\}^{-1} (\boldsymbol{\eta}_S + \mathbf{r}_S - \boldsymbol{\tau}_S) + \boldsymbol{\eta}_{Sc} + \mathbf{r}_{Sc},\end{aligned}$$

where  $\mathbf{r}_{Sc}$  is a  $(d_n - s_n) \times 1$  vector such that its  $j$ -th element equals to

$$(\boldsymbol{\theta}_S - \boldsymbol{\theta}_S^*)^T \nabla_{\boldsymbol{\theta}_S}^2 \{ \mathbb{E}[\nabla_{\boldsymbol{\theta}_{Sc}} \ell(\tilde{\boldsymbol{\theta}})] \}_j (\boldsymbol{\theta}_S - \boldsymbol{\theta}_S^*),$$

and  $\tilde{\boldsymbol{\theta}}$  is a vector lying on the line segment joining  $\widehat{\boldsymbol{\theta}}$  and  $\boldsymbol{\theta}^*$ . Then,

$$\begin{aligned}\|\nabla_{\boldsymbol{\theta}_{Sc}} \ell(\widehat{\boldsymbol{\theta}})\|_\infty &\leq \|\mathbb{E}[\nabla_{\boldsymbol{\theta}_{Sc} \boldsymbol{\theta}_S} \ell(\boldsymbol{\theta}^*)] \left\{ \mathbb{E}[\nabla_{\boldsymbol{\theta}_S}^2 \ell(\boldsymbol{\theta}^*)] \right\}^{-1}\|_\infty (\|\boldsymbol{\eta}_S\|_\infty + \|\mathbf{r}_S\|_\infty + \|\boldsymbol{\tau}_S\|_\infty) \\ &\quad + \|\boldsymbol{\eta}_{Sc}\|_\infty + \|\mathbf{r}_{Sc}\|_\infty.\end{aligned}\tag{S.13}$$

Similarly as (S.11), we have  $\|\mathbf{r}_{Sc}\|_\infty = O(s_n n^{-2\delta})$ . By (S.11), (S.12), condition (C6) and the stated choice of  $\lambda_1$  and  $\lambda_2$ , we have

$$\begin{aligned}&\lambda_{ln}^{-1} \|\mathbb{E}[\nabla_{\boldsymbol{\theta}_{Sc} \boldsymbol{\theta}_S} \ell(\boldsymbol{\theta}^*)] \left\{ \mathbb{E}[\nabla_{\boldsymbol{\theta}_S}^2 \ell(\boldsymbol{\theta}^*)] \right\}^{-1}\|_\infty (\|\boldsymbol{\eta}_S\|_\infty + \|\mathbf{r}_S\|_\infty) + \lambda_{ln}^{-1} \|\boldsymbol{\eta}_{Sc}\|_\infty + \lambda_{ln}^{-1} \|\mathbf{r}_{Sc}\|_\infty \\ &= o(\lambda_{ln}^{-1} n^\xi \{s_n^{3/2} b_n / \sqrt{n} + \sqrt{(\log n)/n} + s_n n^{-2\delta}\}) + O(\lambda_{ln}^{-1} n^\xi \{s_n^{3/2} b_n / \sqrt{n} + \sqrt{(\log d_n)/n}\}) \\ &\quad + O(\lambda_{ln}^{-1} s_n n^{-2\delta}) \\ &= o(1).\end{aligned}$$

The dominating term in (S.13) has

$$\lambda_1^{-1} \|\mathbb{E}[\nabla_{\boldsymbol{\theta}_{Sc}}^2 \ell(\boldsymbol{\theta}^*)] \left\{ \mathbb{E}[\nabla_{\boldsymbol{\theta}_S}^2 \ell(\boldsymbol{\theta}^*)] \right\}^{-1}\|_\infty \|\boldsymbol{\tau}_S\|_\infty < \lambda_1^{-1} \frac{\rho'(0+)}{\rho'(b_n)} \lambda_1 \rho'(b_n) < \rho'(0+),$$

Therefore (S.7) holds. By a similar argument, we can also prove (S.8). This completes the proof of statement [2].  $\square$

## References

Afsari, B., Fertig, E. J., Geman, D., and Marchionni, L. (2015). SwitchBox: an R package for K-top scoring pairs classifier development. *Bioinformatics* **31**, 273–274.

- Fan, J. and Lv, J. (2011). Nonconcave penalized likelihood with NP-dimensionality. *Information Theory, IEEE Transactions* **57**, 5467–5484.
- Massart, P. (2007). *Concentration inequalities and model selection*, volume 6. Springer.
- Van der Vaart, A. W. (2000). *Asymptotic statistics*, volume 3. Cambridge university press.
- Vrahatis, M. N. (1989). A short proof and a generalization of miranda’s existence theorem. *Proceedings of the American Mathematical Society* **107**, 701–703.
